# Supplementary material for: JEAN: Joint Expression and Audio-guided NeRF-based Talking Face Generation
Source: arXiv:2409.12156 source file (2024-09-18)
Supplement: Supplementary file 1 [file testing.tex]

% While comparing with methods like AD-NeRF~\cite{guo2021adnerf} and NeRFace~\cite{nerface}, we train separate networks on each tested identity and use pretrained networks for the rest of the methods. 
\documentclass{bmvc2k}
\graphicspath{{\subfix{../images/}}}
\begin{document}
$$N ... 1$$
\noindent
$1$

\noindent
$.$

\noindent
$.$

\noindent
$.$

\noindent
$N$
\end{document}
